# Supplementary material for: MTNT: A Testbed for Machine Translation of Noisy Text
Source: arXiv:1809.00388 source file (2018-09-02)
Supplement: Supplementary file 1 [file 9_supplemental.tex]

\section{Supplemental Material}
\label{sec:supplemental}

See Table \ref{tab:compare_ngrams}.
